# Supplementary material for: Analysis of the heat transfer fluctuations in the Rayleigh-B\'enard convection of concentrated emulsions with finite-size droplets
Source: arXiv:2306.02404 ancillary file (2023-08-10)
Supplement: Supplementary file 1 [file supplementary.pdf]

# SUPPLEMENTARY MATERIAL FOR: Analysis of the heat transfer fluctuations in the Rayleigh-Bénard convection of concentrated emulsions with finite-size droplets


Francesca Pelusi,[1,*] Stefano Ascione,[2] Mauro Sbragaglia,[3] and Massimo Bernaschi[1]

[1] *Istituto per le Applicazioni del Calcolo, CNR - Via dei Taurini 19, 00185 Rome, Italy*

[2] *Department of Physics, Tor Vergata University of Rome - Via della Ricerca Scientifica 1, 00133 Rome, Italy*

[3] *Department of Physics & INFN, Tor Vergata University of Rome, Via della Ricerca Scientifica 1, 00133 Rome, Italy*



(Dated: June 4, 2023)


## I. RHEOLOGY

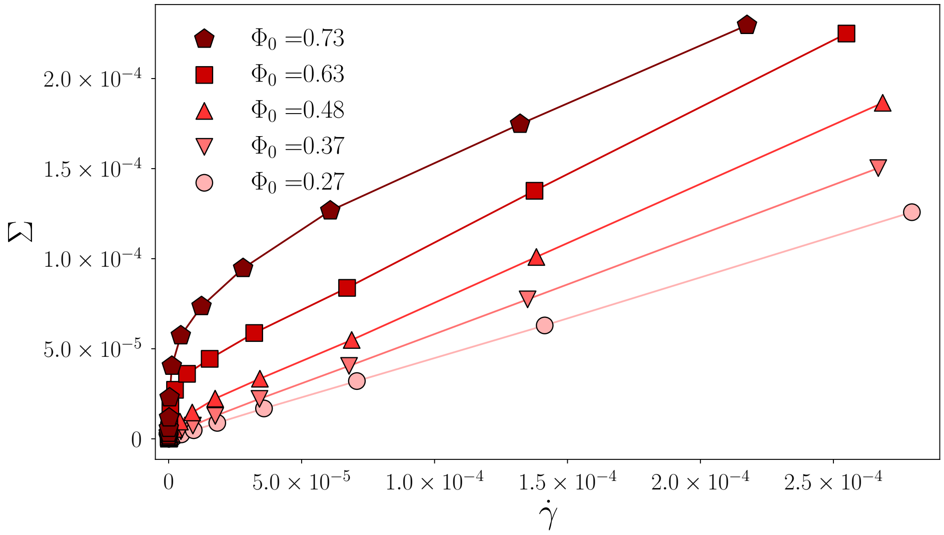


FIG. 1. Rheological characterization of emulsion systems explored in this work, from diluted ($\Phi_0 = 0.27$) to highly packed emulsions ($\Phi_0 = 0.73$).

In order to characterize the rheological nature of the emulsion systems explored in this work, we performed a Couette experiment where constant and opposite velocities are imposed at the walls along the $x$- direction ($u_{x,wall}(y = \pm H/2, t) = \pm u_{wall}$). For each droplet concentration $\Phi_0$, we measure the stress $\Sigma$ at varying $u_{wall}$, resulting in different values of the the shear rate $\dot{\gamma} = 2u_{wall}/H$. Results are shown in Fig. 1. Flow curves highlight how different is the mechanical response of these emulsions, moving from Newtonian (diluted cases) to non-Newtonian (more concentrated emulsions).

## II. CORRELATION BETWEEN MESOSCOPIC HEAT TRANSFER FLUCTUATIONS AND DROPLET LOCALISATION

In the main text we discuss about the correlation between droplet localisation, expressed in terms of the $y$-coordinate of its center-of-mass-position ($Y_i$), and its corresponding heat transfer fluctuation $\mathrm{Nu}_i^{*,(drop)}$ (cfr. Fig. 4 of the main text). We observe that $\mathrm{Nu}_i^{*,(drop)}$ exhibits an intermittent behaviour and that there is an evident correlation between "bursts" in the droplet heat transfer fluctuation and the spatial approach-to/departure-from a wall. We also claim


* f.pelusi@iac.cnr.it

that a variation in the period of oscillation of $Y_i$ is related to a layer change by the selected drop. In order to help the reader in catching this phenomenon, we include three videos, labelled as Phi027.mp4, Phi048.mp4, and Phi073.mp4, showing an animation of Fig. 4 of the main text.
